# Supplementary material for: Enhancing predictive imaging biomarker discovery through treatment effect analysis
Source: arXiv:2406.02534 source file (2024-12-09)
Supplement: Supplementary file 1 [file figure_appendix_XAI.pdf]

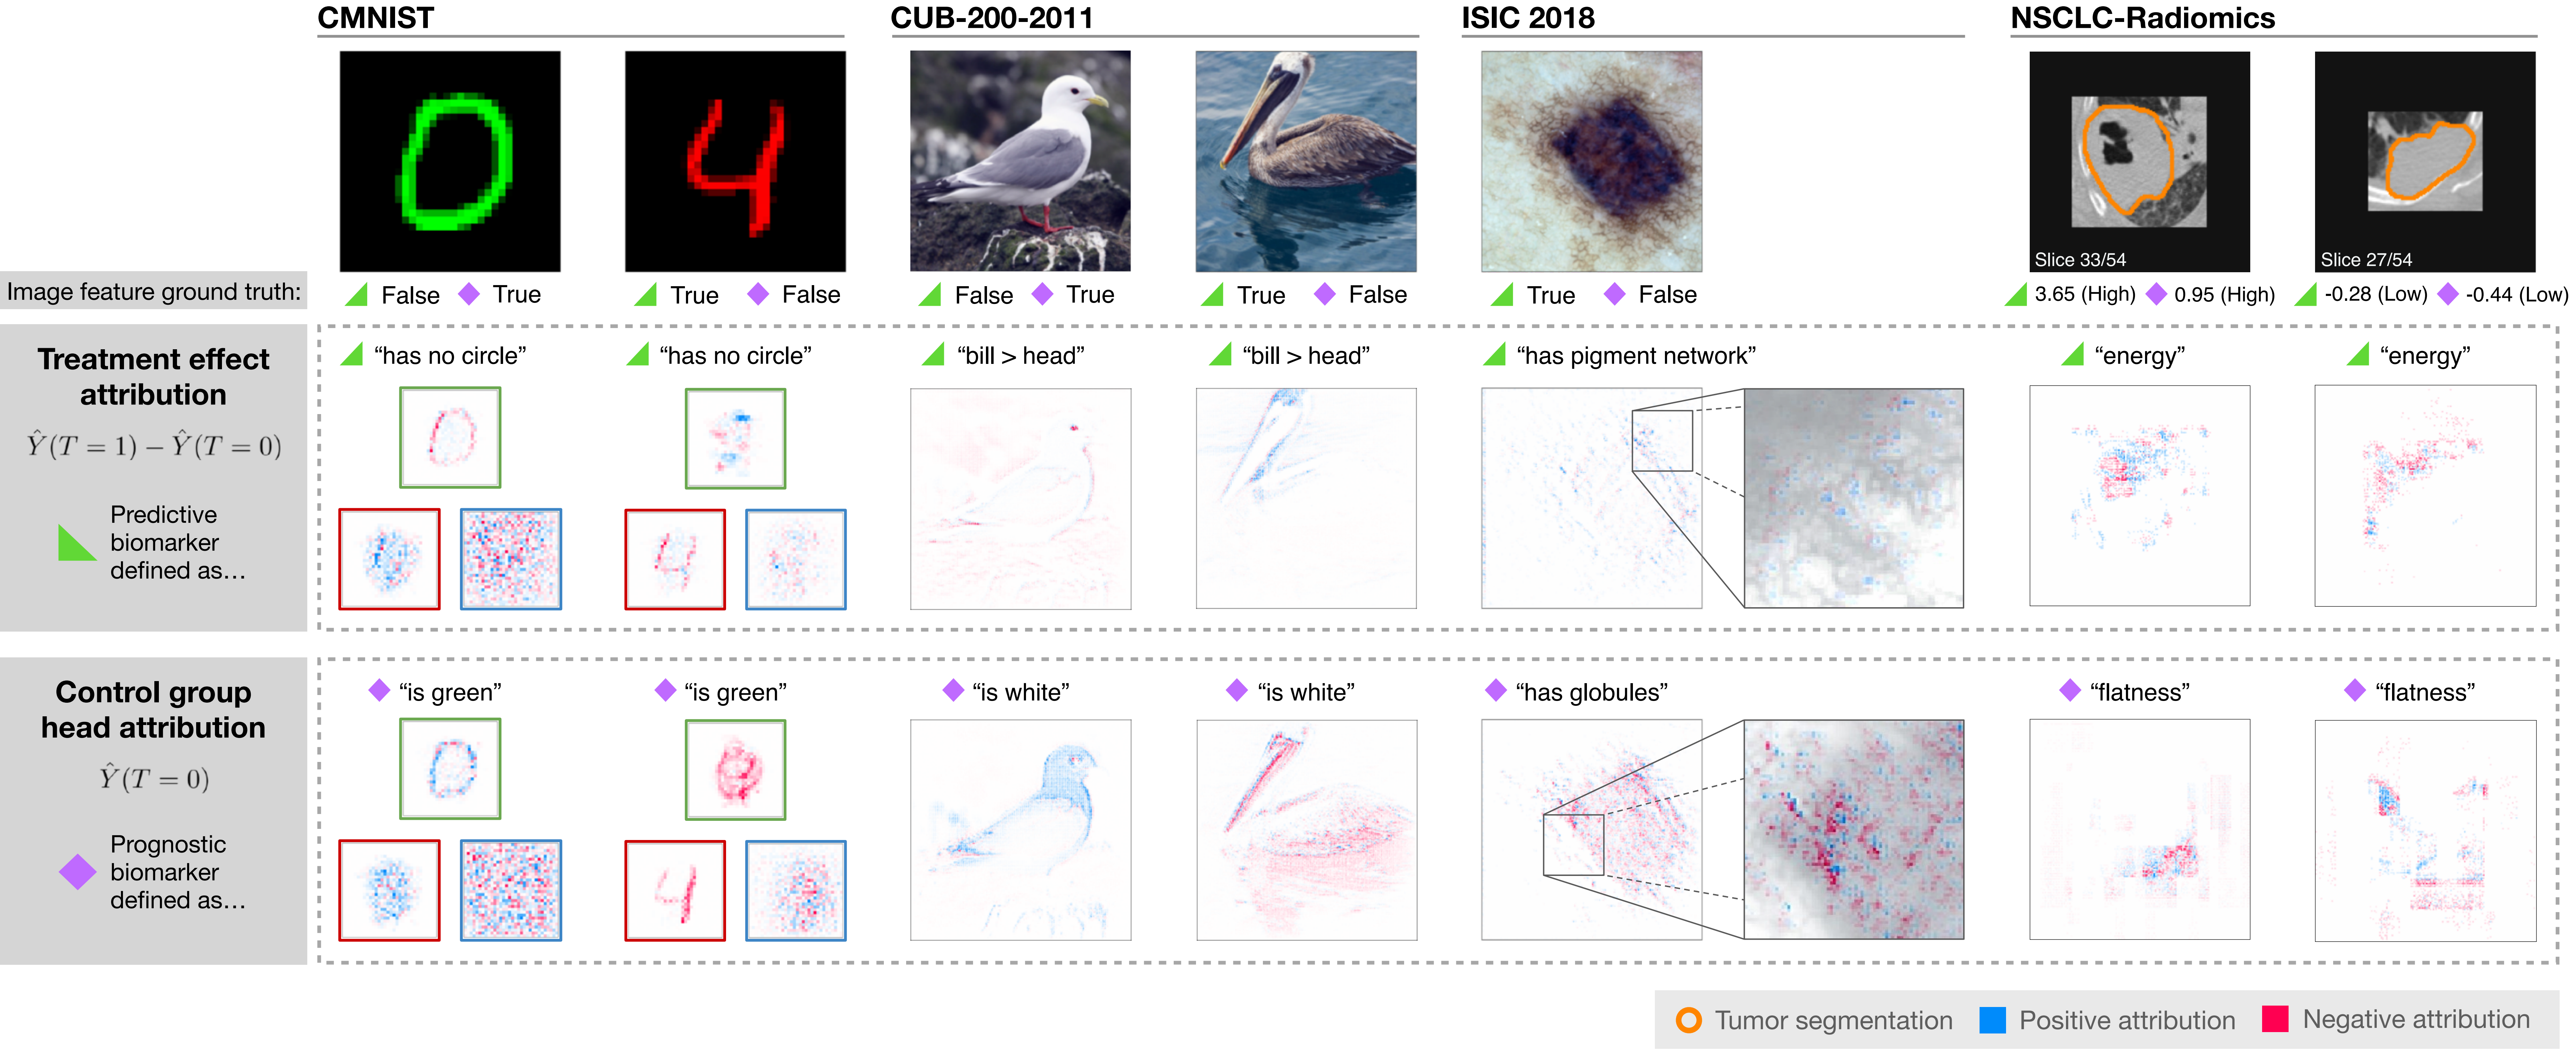

CMNIST
CUB-200-2011
ISIC 2018
NSCLC-Radiomics
Image feature ground truth:
False True
True False
False True
True False
True False
Slice 33/54
Slice 27/54
3.65 (High) 0.95 (High)
-0.28 (Low) -0.44 (Low)
Treatment effect attribution
$\hat{Y}(T=1) - \hat{Y}(T=0)$
Predictive biomarker defined as…
"has no circle"
"has no circle"
"bill > head"
"bill > head"
"has pigment network"
"energy"
"energy"
Control group head attribution
$\hat{Y}(T=0)$
Prognostic biomarker defined as…
"is green"
"is green"
"is white"
"is white"
"has globules"
"flatness"
"flatness"
Tumor segmentation
Positive attribution
Negative attribution

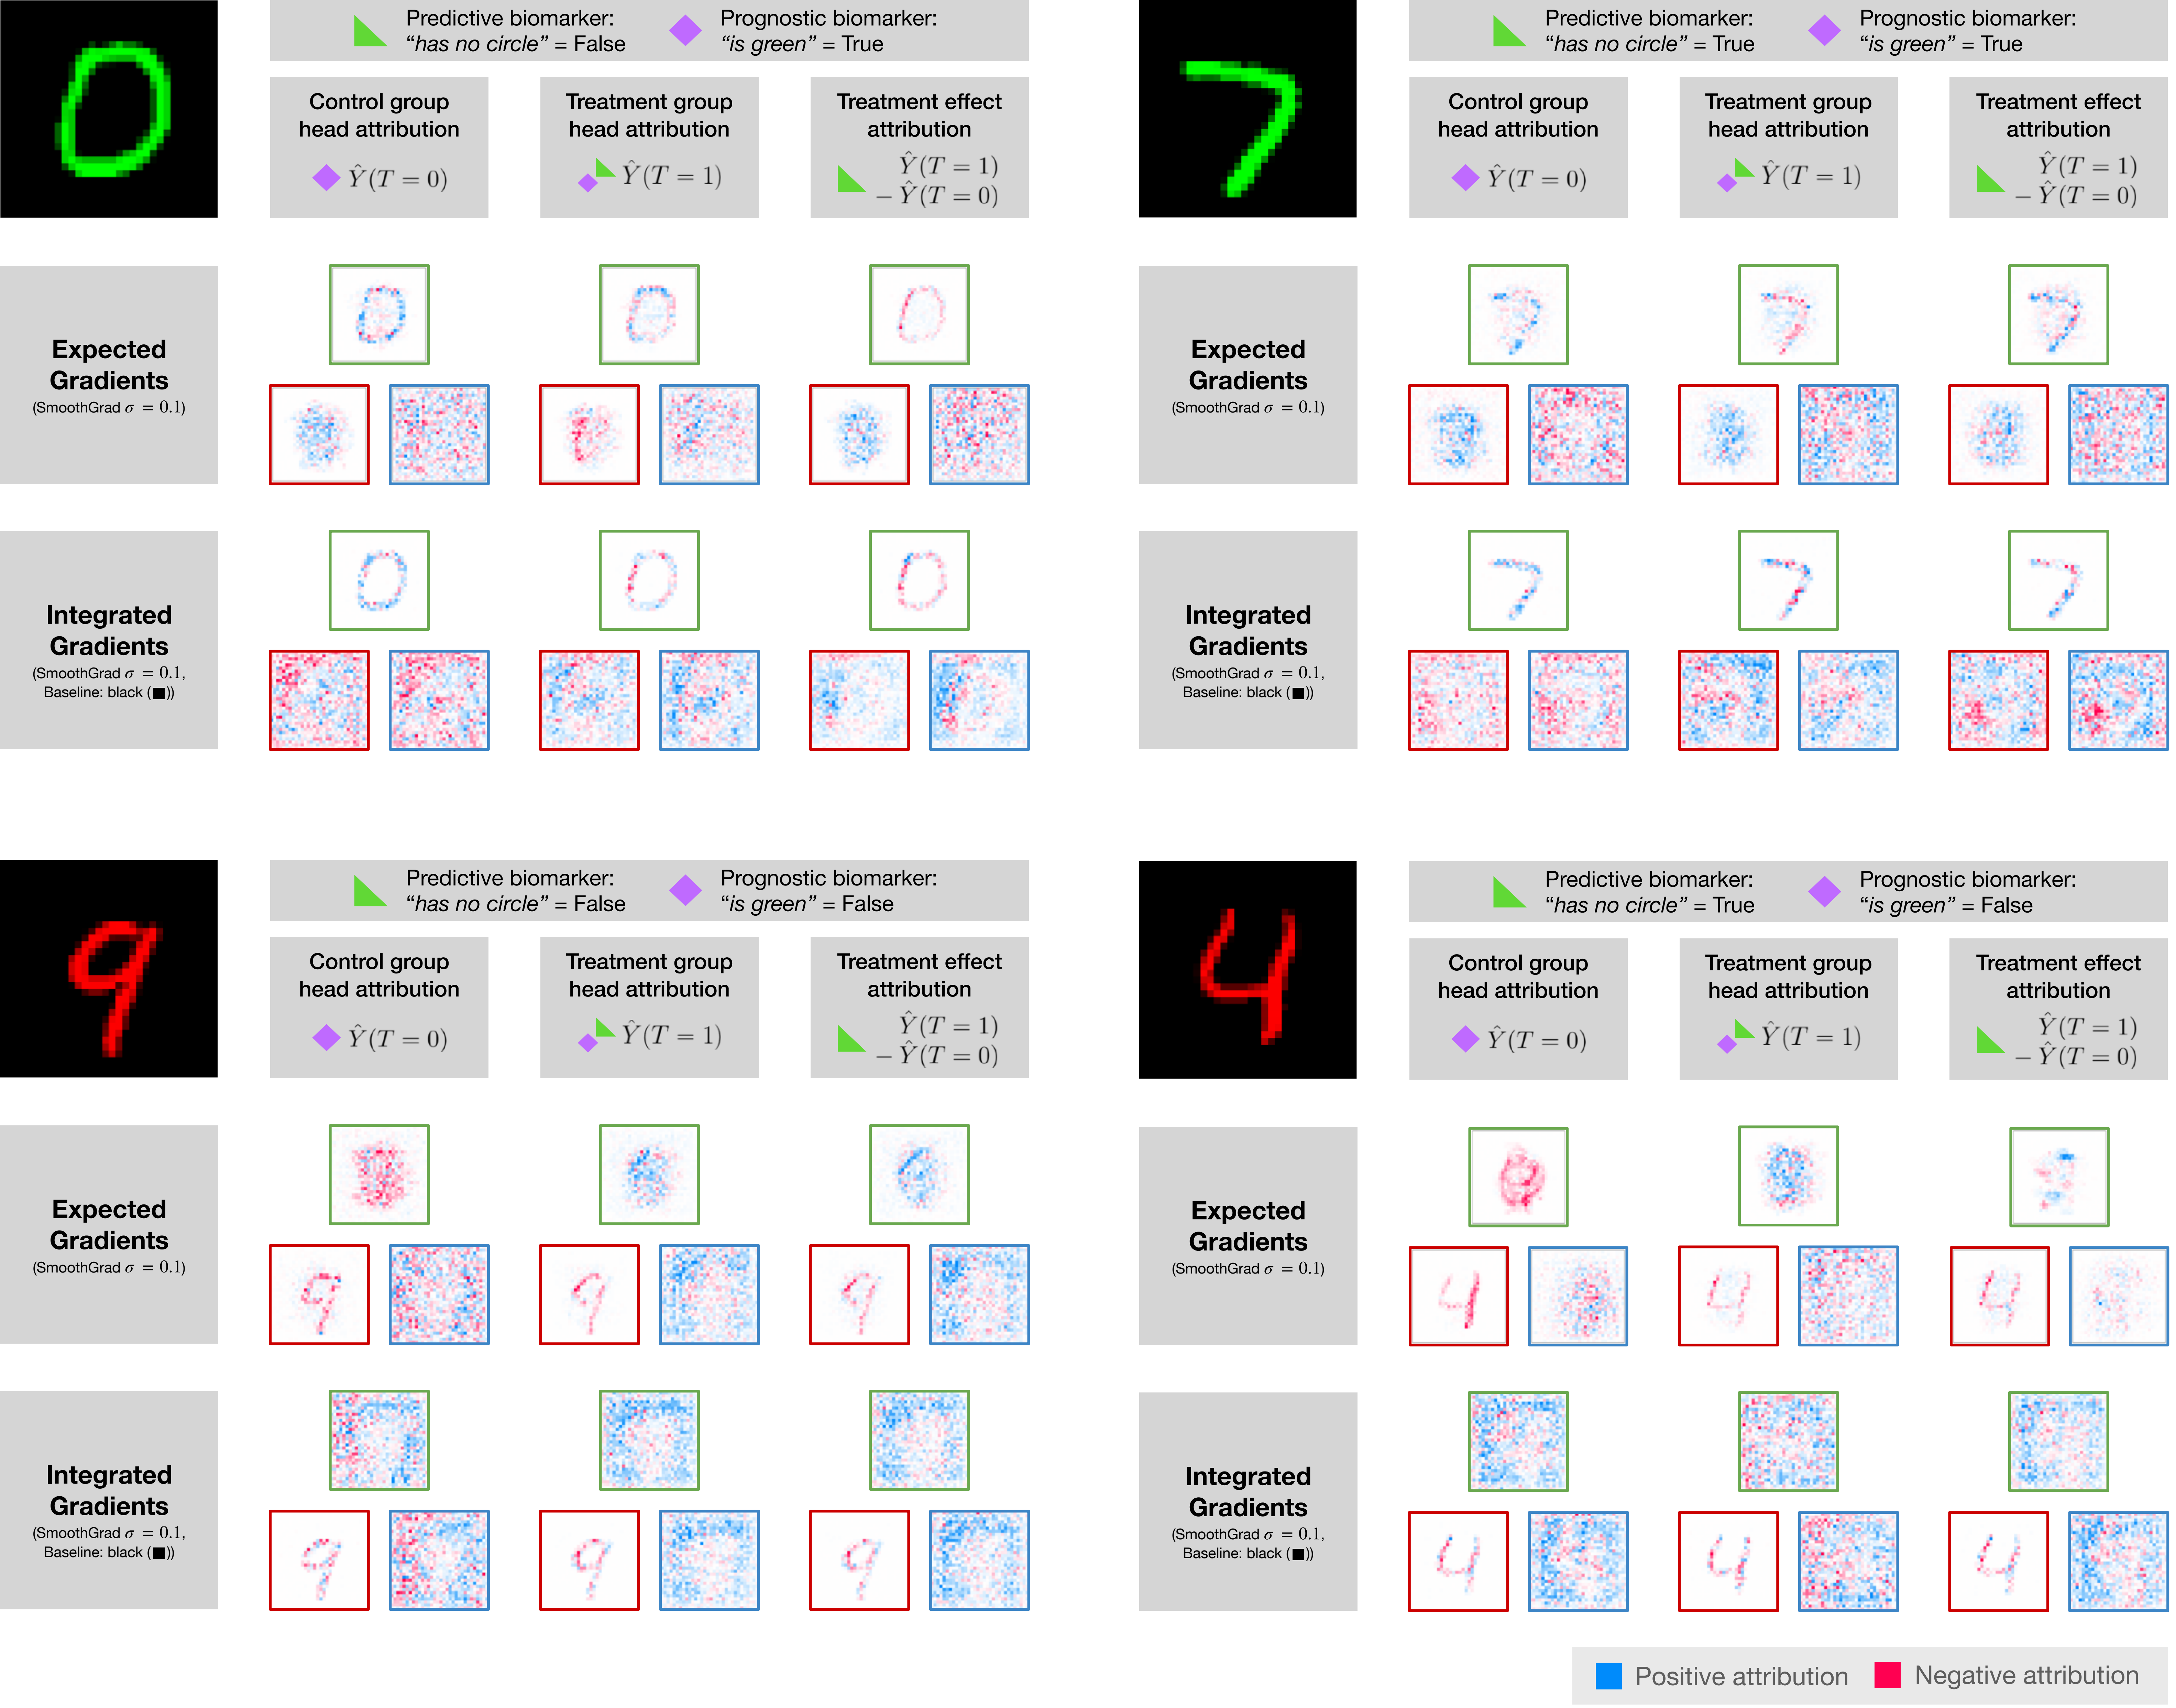

Predictive biomarker: "has no circle" = False
Prognostic biomarker: "is green" = True
Control group head attribution
Ŷ(T = 0)
Treatment group head attribution
Ŷ(T = 1)
Treatment effect attribution
Ŷ(T = 1) − Ŷ(T = 0)
Expected Gradients
(SmoothGrad σ = 0.1)
Integrated Gradients
(SmoothGrad σ = 0.1, Baseline: black (■))
Predictive biomarker: "has no circle" = True
Prognostic biomarker: "is green" = True
Predictive biomarker: "has no circle" = False
Prognostic biomarker: "is green" = False
Predictive biomarker: "has no circle" = True
Prognostic biomarker: "is green" = False
Positive attribution
Negative attribution

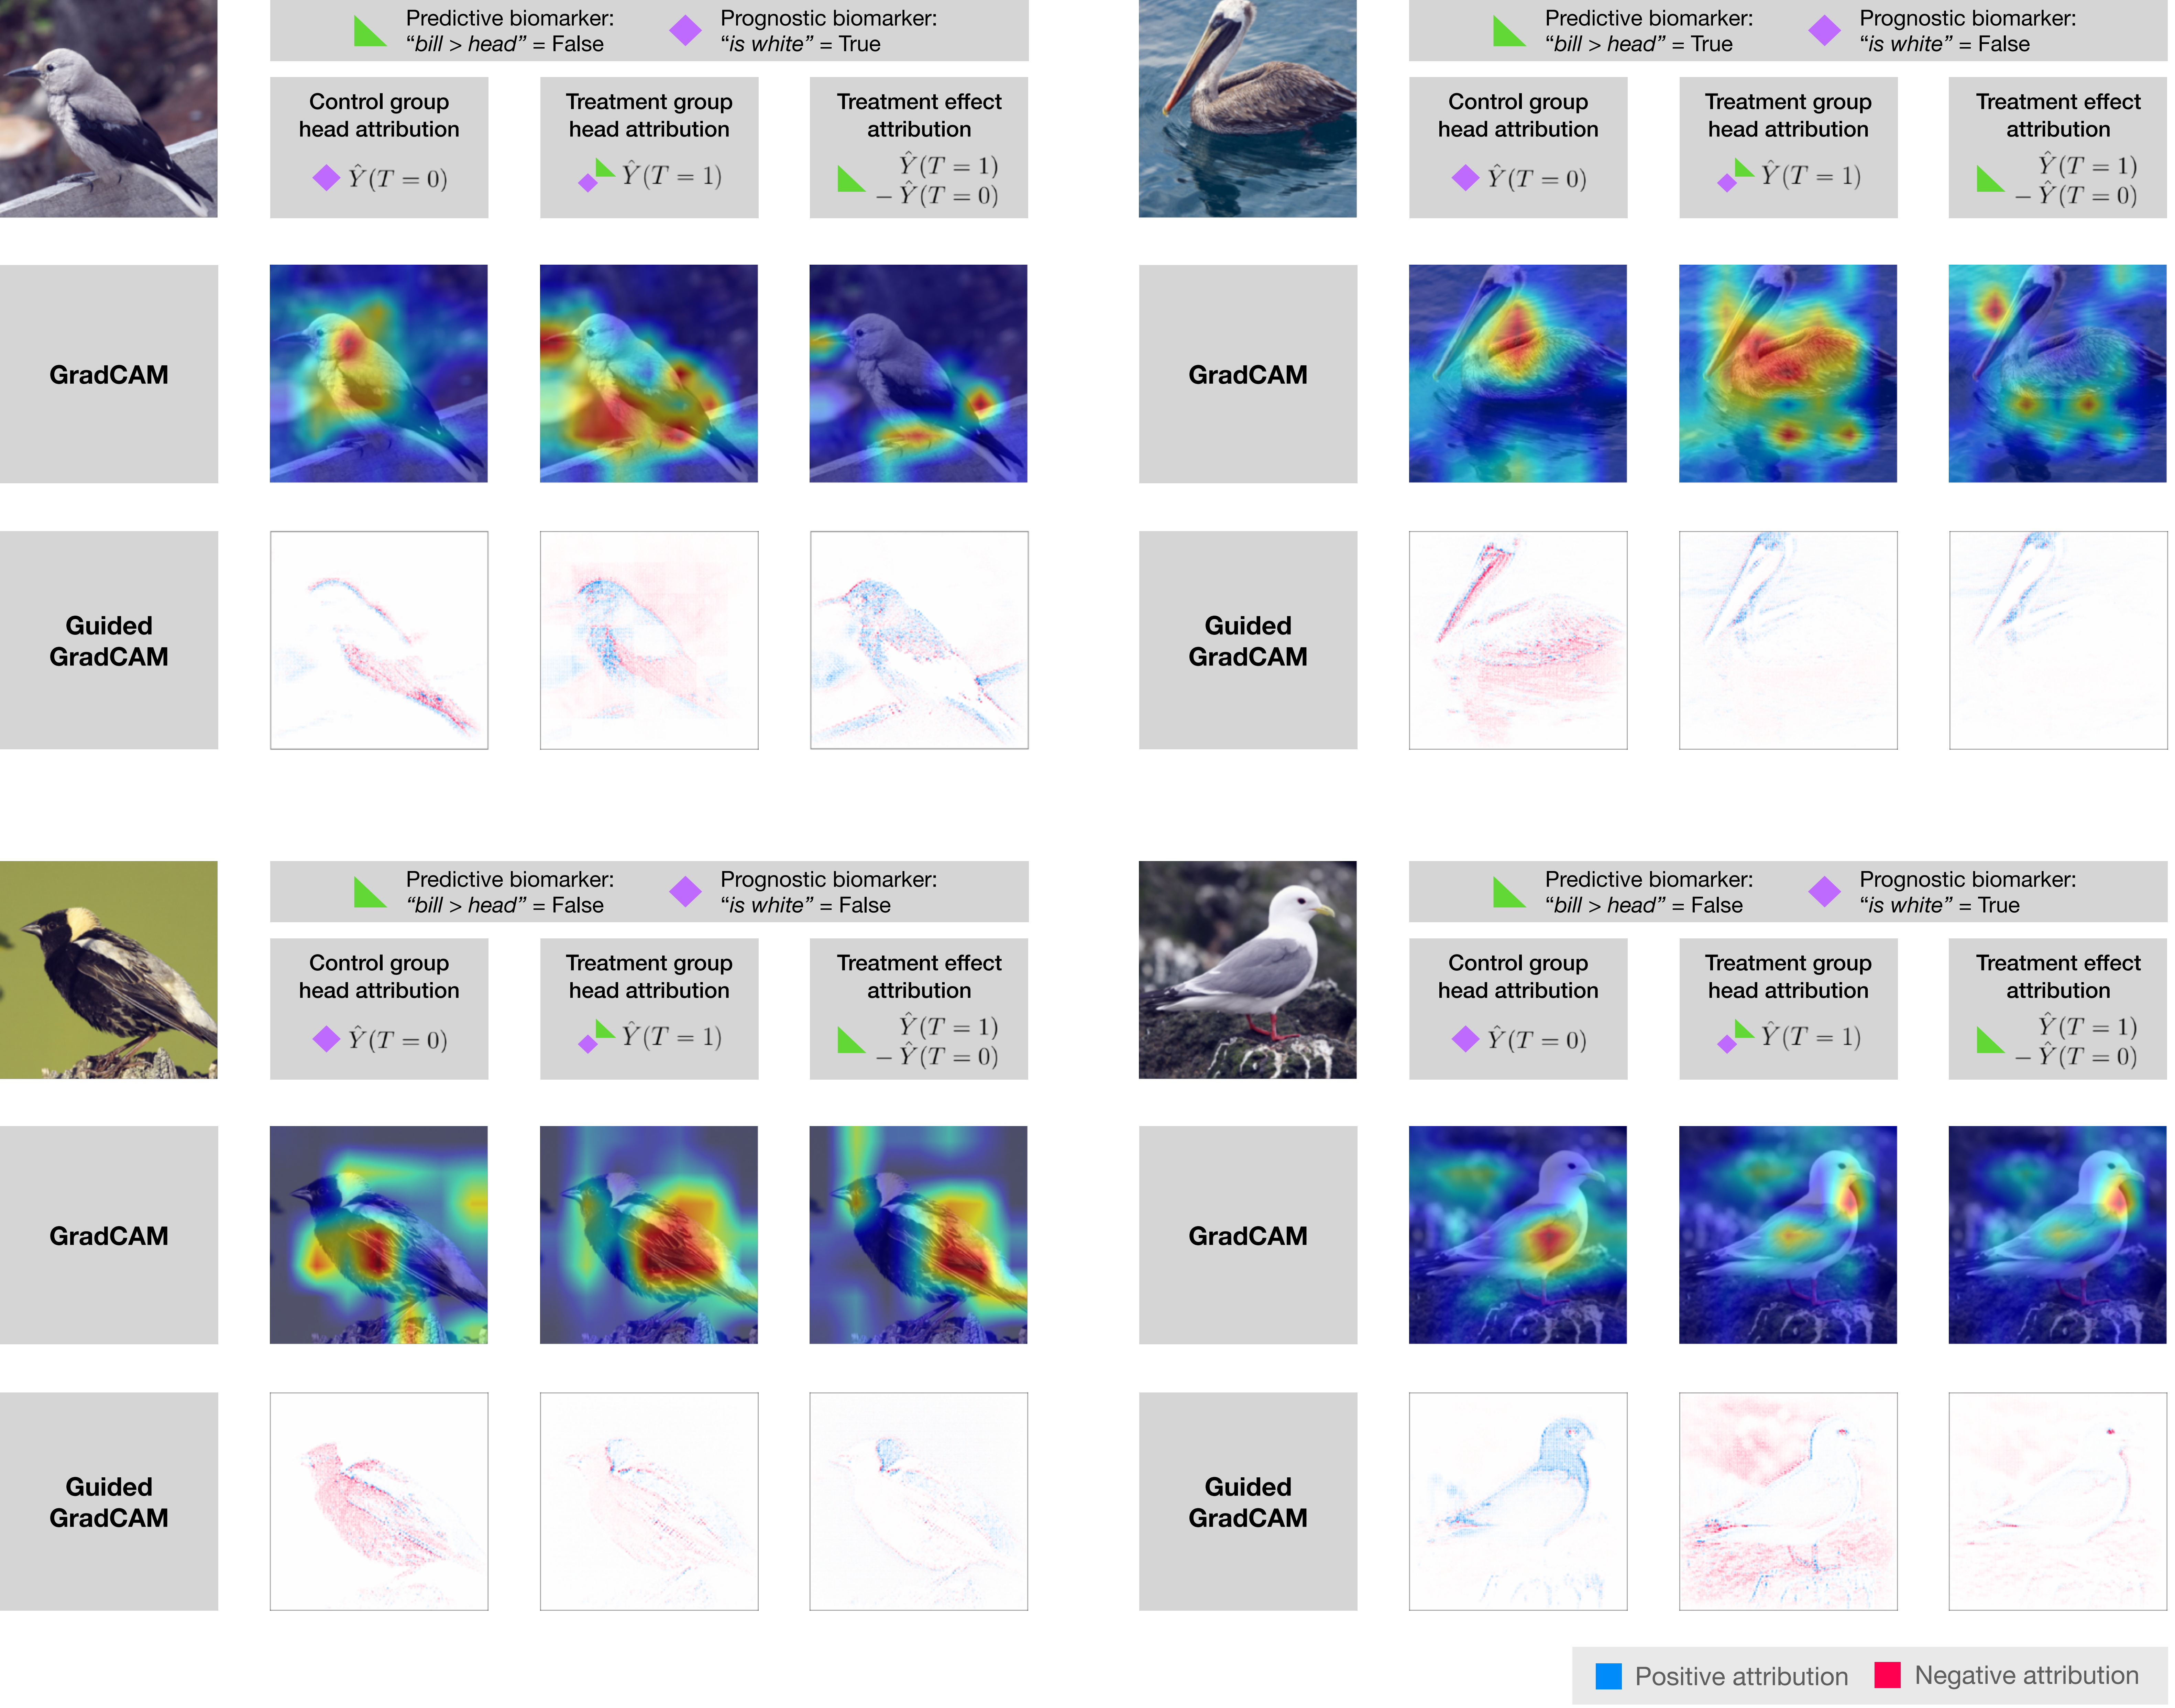

Predictive biomarker: "bill > head" = False
Prognostic biomarker: "is white" = True
Control group head attribution
$\hat{Y}(T=0)$
Treatment group head attribution
$\hat{Y}(T=1)$
Treatment effect attribution
$\hat{Y}(T=1) - \hat{Y}(T=0)$
GradCAM
Guided GradCAM
Predictive biomarker: "bill > head" = True
Prognostic biomarker: "is white" = False
Control group head attribution
$\hat{Y}(T=0)$
Treatment group head attribution
$\hat{Y}(T=1)$
Treatment effect attribution
$\hat{Y}(T=1) - \hat{Y}(T=0)$
GradCAM
Guided GradCAM
Predictive biomarker: "bill > head" = False
Prognostic biomarker: "is white" = False
Control group head attribution
$\hat{Y}(T=0)$
Treatment group head attribution
$\hat{Y}(T=1)$
Treatment effect attribution
$\hat{Y}(T=1) - \hat{Y}(T=0)$
GradCAM
Guided GradCAM
Predictive biomarker: "bill > head" = False
Prognostic biomarker: "is white" = True
Control group head attribution
$\hat{Y}(T=0)$
Treatment group head attribution
$\hat{Y}(T=1)$
Treatment effect attribution
$\hat{Y}(T=1) - \hat{Y}(T=0)$
GradCAM
Guided GradCAM
Positive attribution
Negative attribution

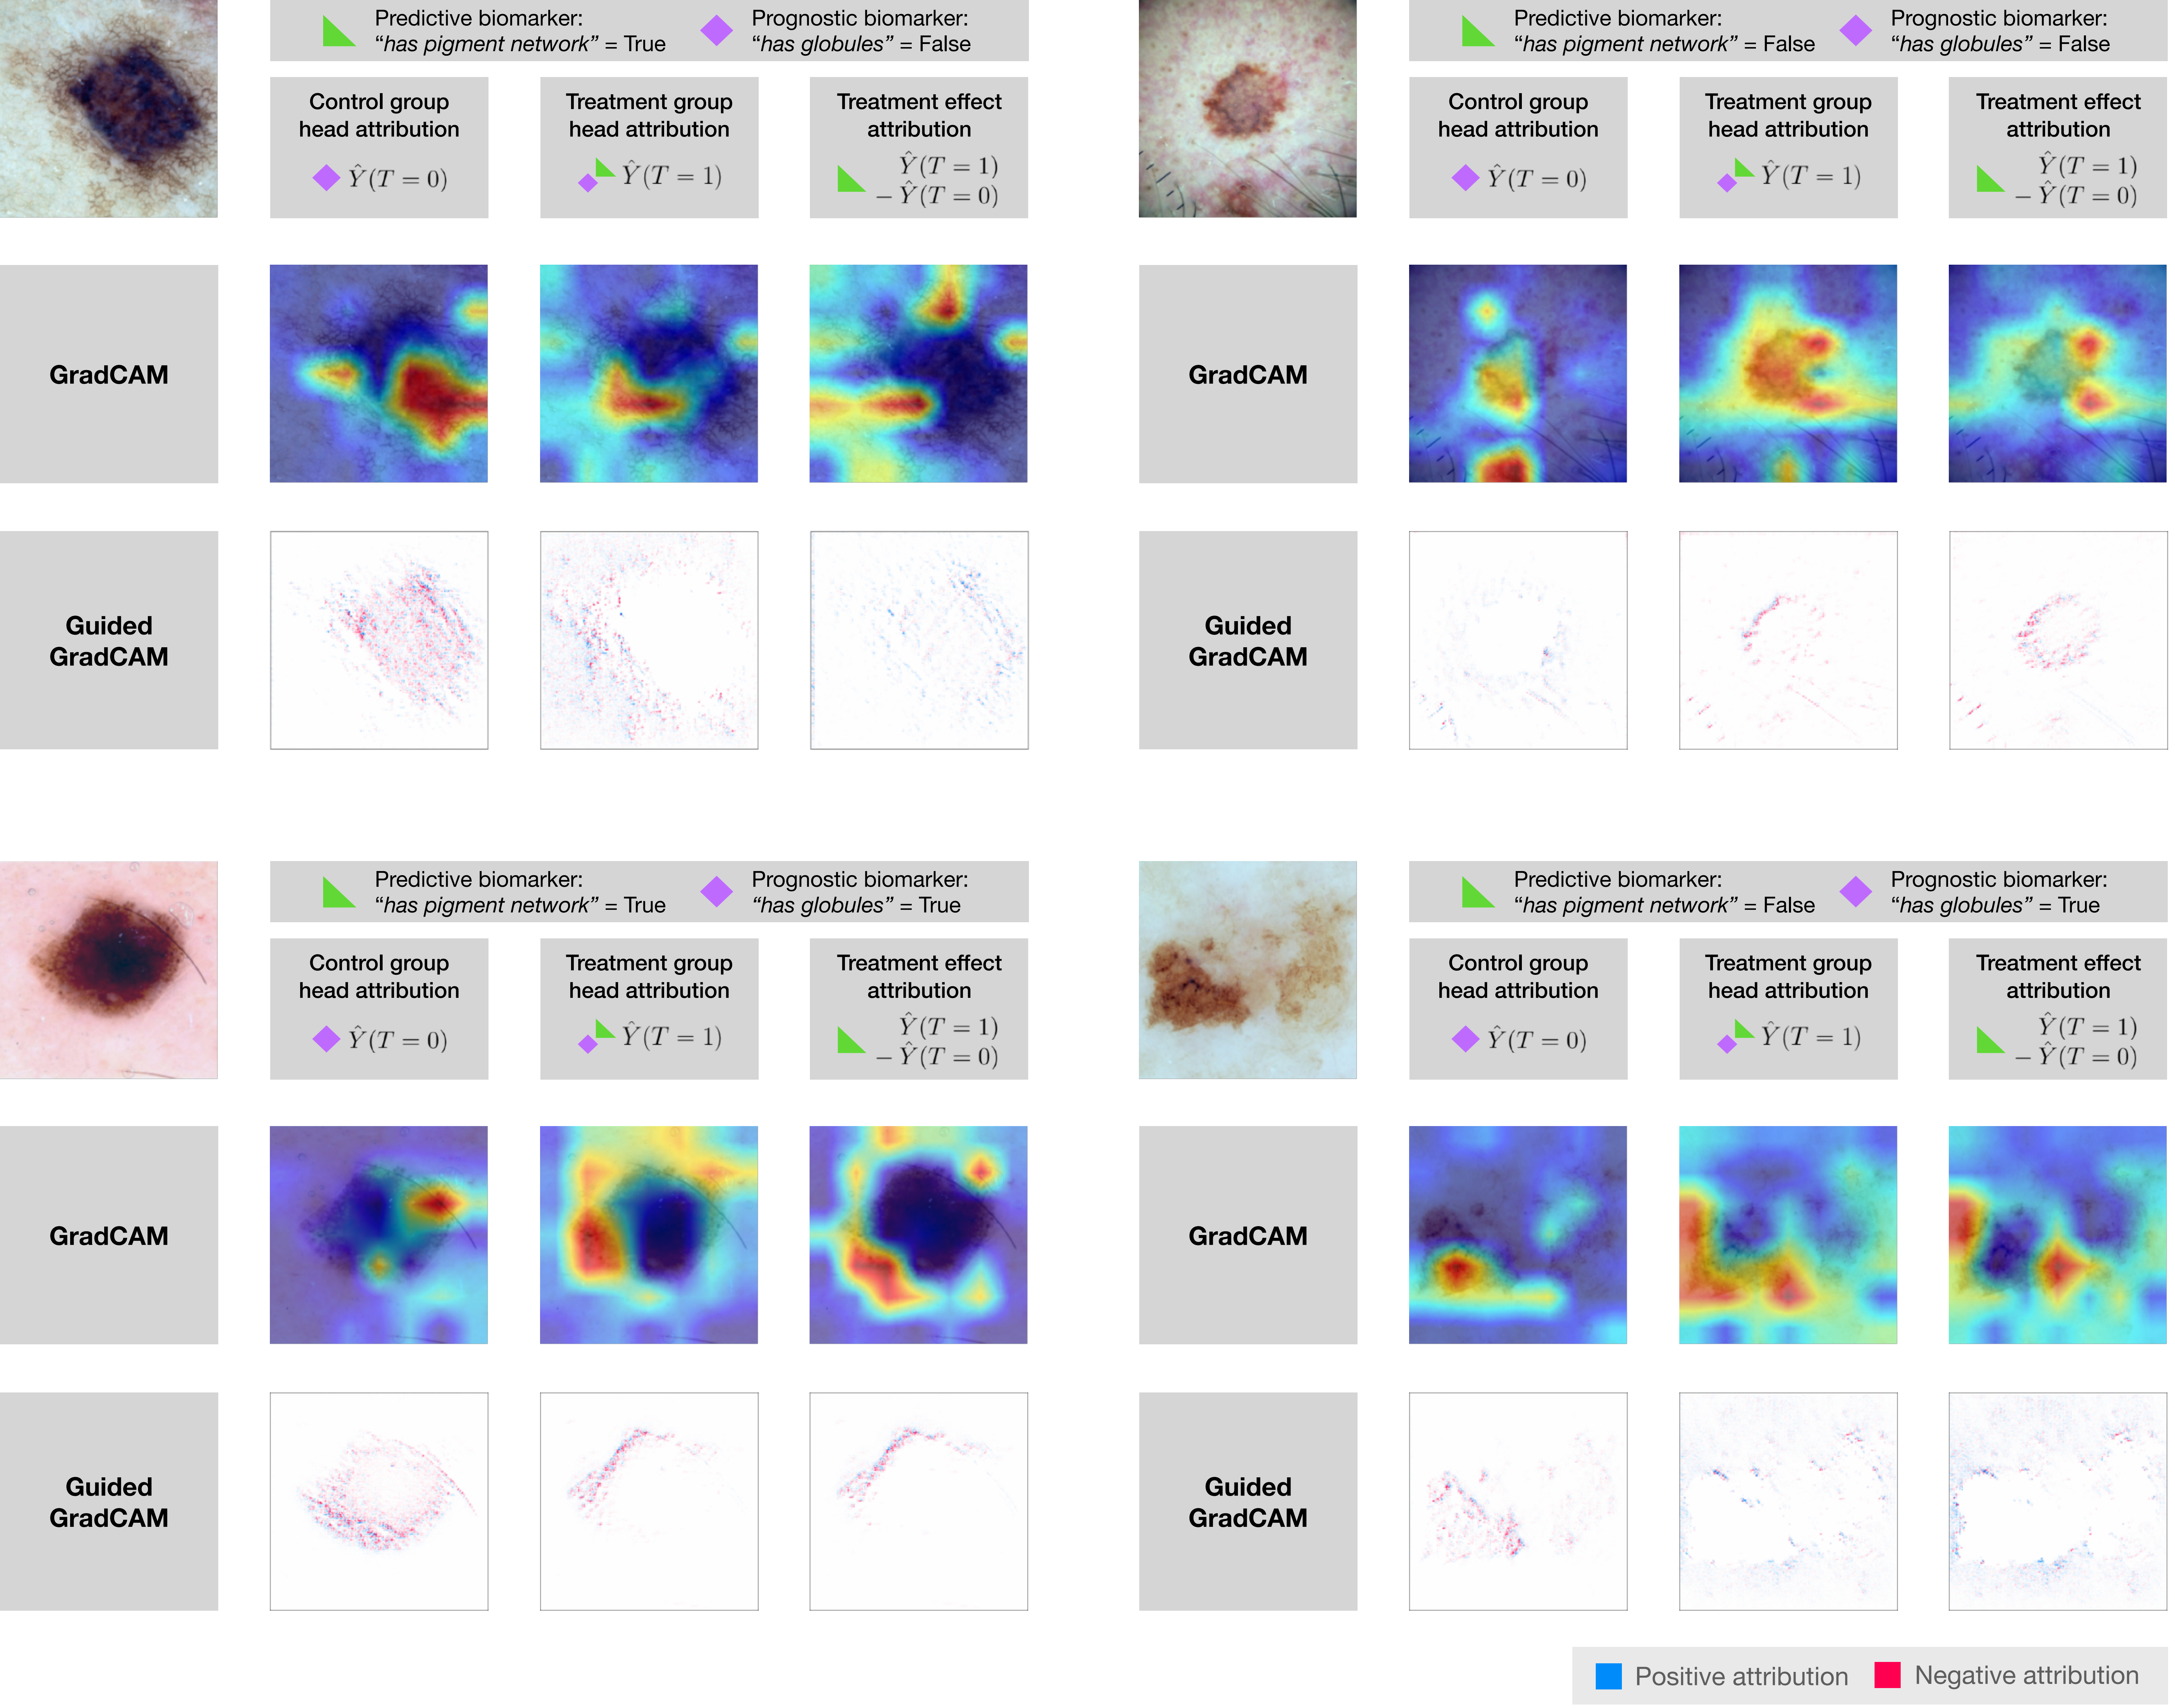

Predictive biomarker: "has pigment network" = True
Prognostic biomarker: "has globules" = False
Control group head attribution
$\hat{Y}(T=0)$
Treatment group head attribution
$\hat{Y}(T=1)$
Treatment effect attribution
$\hat{Y}(T=1) - \hat{Y}(T=0)$
GradCAM
Guided GradCAM
Predictive biomarker: "has pigment network" = False
Prognostic biomarker: "has globules" = False
Predictive biomarker: "has pigment network" = True
Prognostic biomarker: "has globules" = True
Predictive biomarker: "has pigment network" = False
Prognostic biomarker: "has globules" = True
Positive attribution
Negative attribution

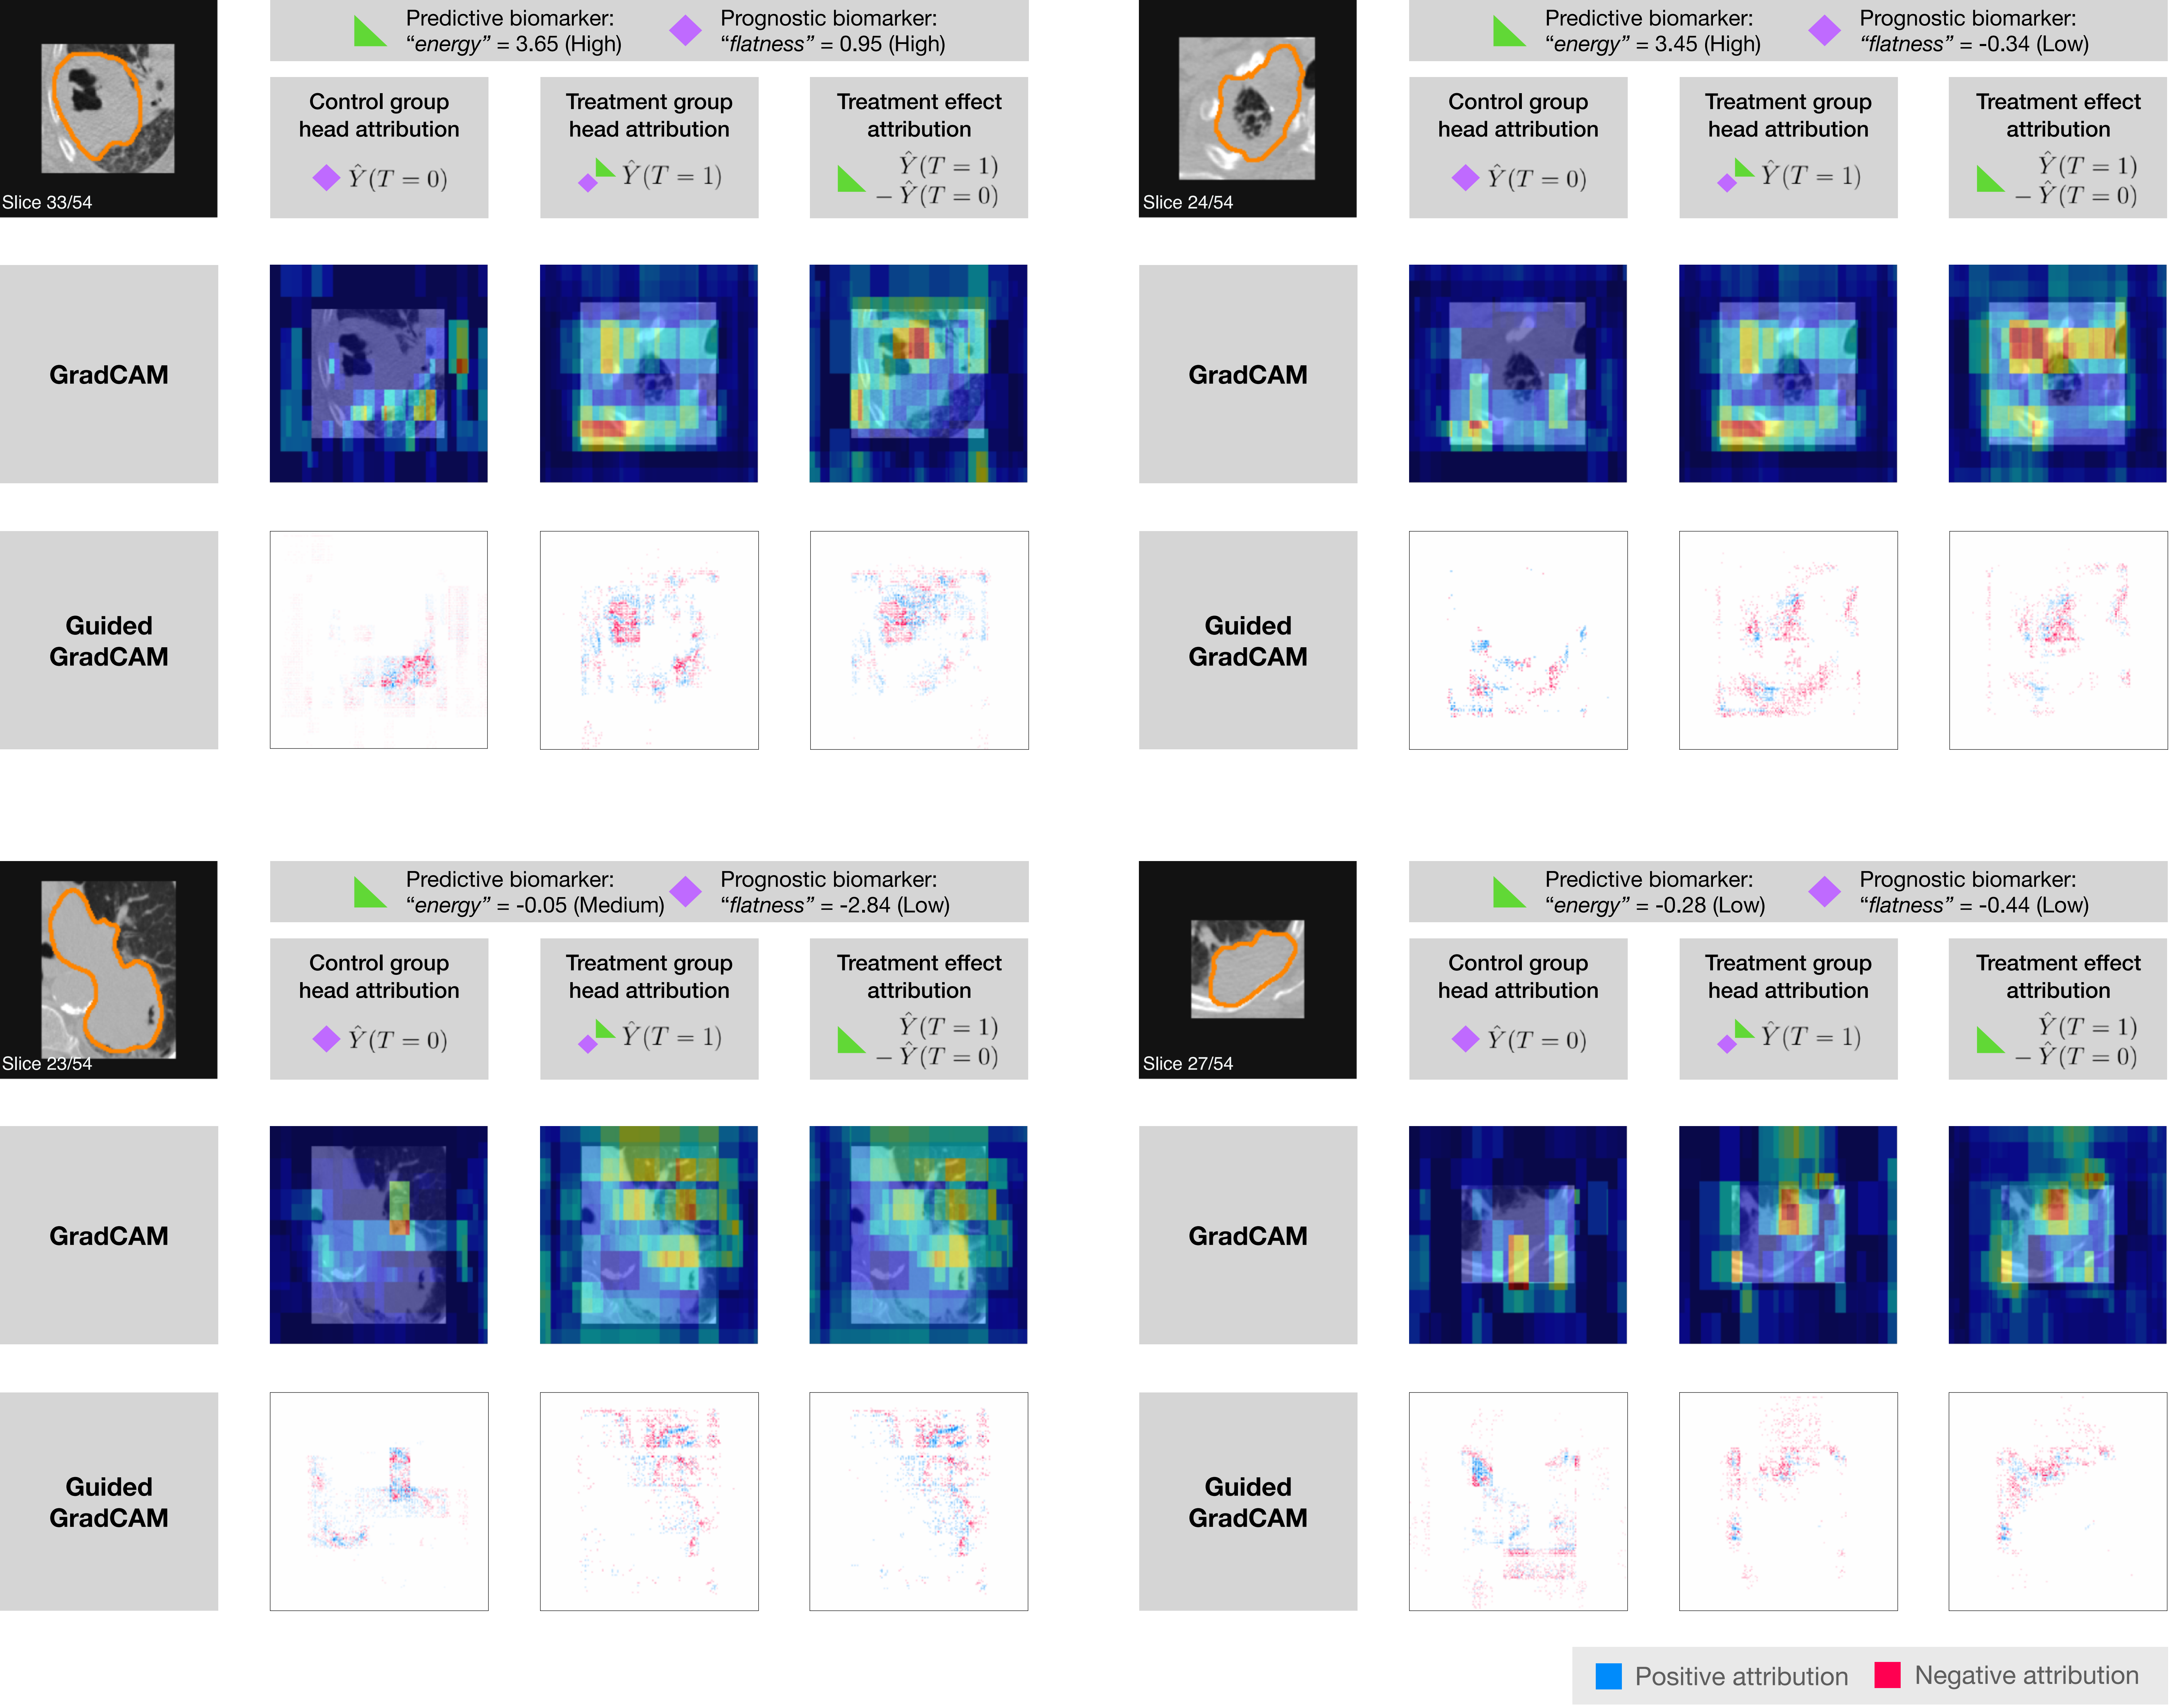
Predictive biomarker: "energy" = 3.65 (High)
Prognostic biomarker: "flatness" = 0.95 (High)
Slice 33/54
Control group head attribution
$\hat{Y}(T=0)$
Treatment group head attribution
$\hat{Y}(T=1)$
Treatment effect attribution
$\hat{Y}(T=1) - \hat{Y}(T=0)$
GradCAM
Guided GradCAM
Predictive biomarker: "energy" = 3.45 (High)
Prognostic biomarker: "flatness" = -0.34 (Low)
Slice 24/54
Control group head attribution
$\hat{Y}(T=0)$
Treatment group head attribution
$\hat{Y}(T=1)$
Treatment effect attribution
$\hat{Y}(T=1) - \hat{Y}(T=0)$
GradCAM
Guided GradCAM
Predictive biomarker: "energy" = -0.05 (Medium)
Prognostic biomarker: "flatness" = -2.84 (Low)
Slice 23/54
Control group head attribution
$\hat{Y}(T=0)$
Treatment group head attribution
$\hat{Y}(T=1)$
Treatment effect attribution
$\hat{Y}(T=1) - \hat{Y}(T=0)$
GradCAM
Guided GradCAM
Predictive biomarker: "energy" = -0.28 (Low)
Prognostic biomarker: "flatness" = -0.44 (Low)
Slice 27/54
Control group head attribution
$\hat{Y}(T=0)$
Treatment group head attribution
$\hat{Y}(T=1)$
Treatment effect attribution
$\hat{Y}(T=1) - \hat{Y}(T=0)$
GradCAM
Guided GradCAM
Positive attribution
Negative attribution

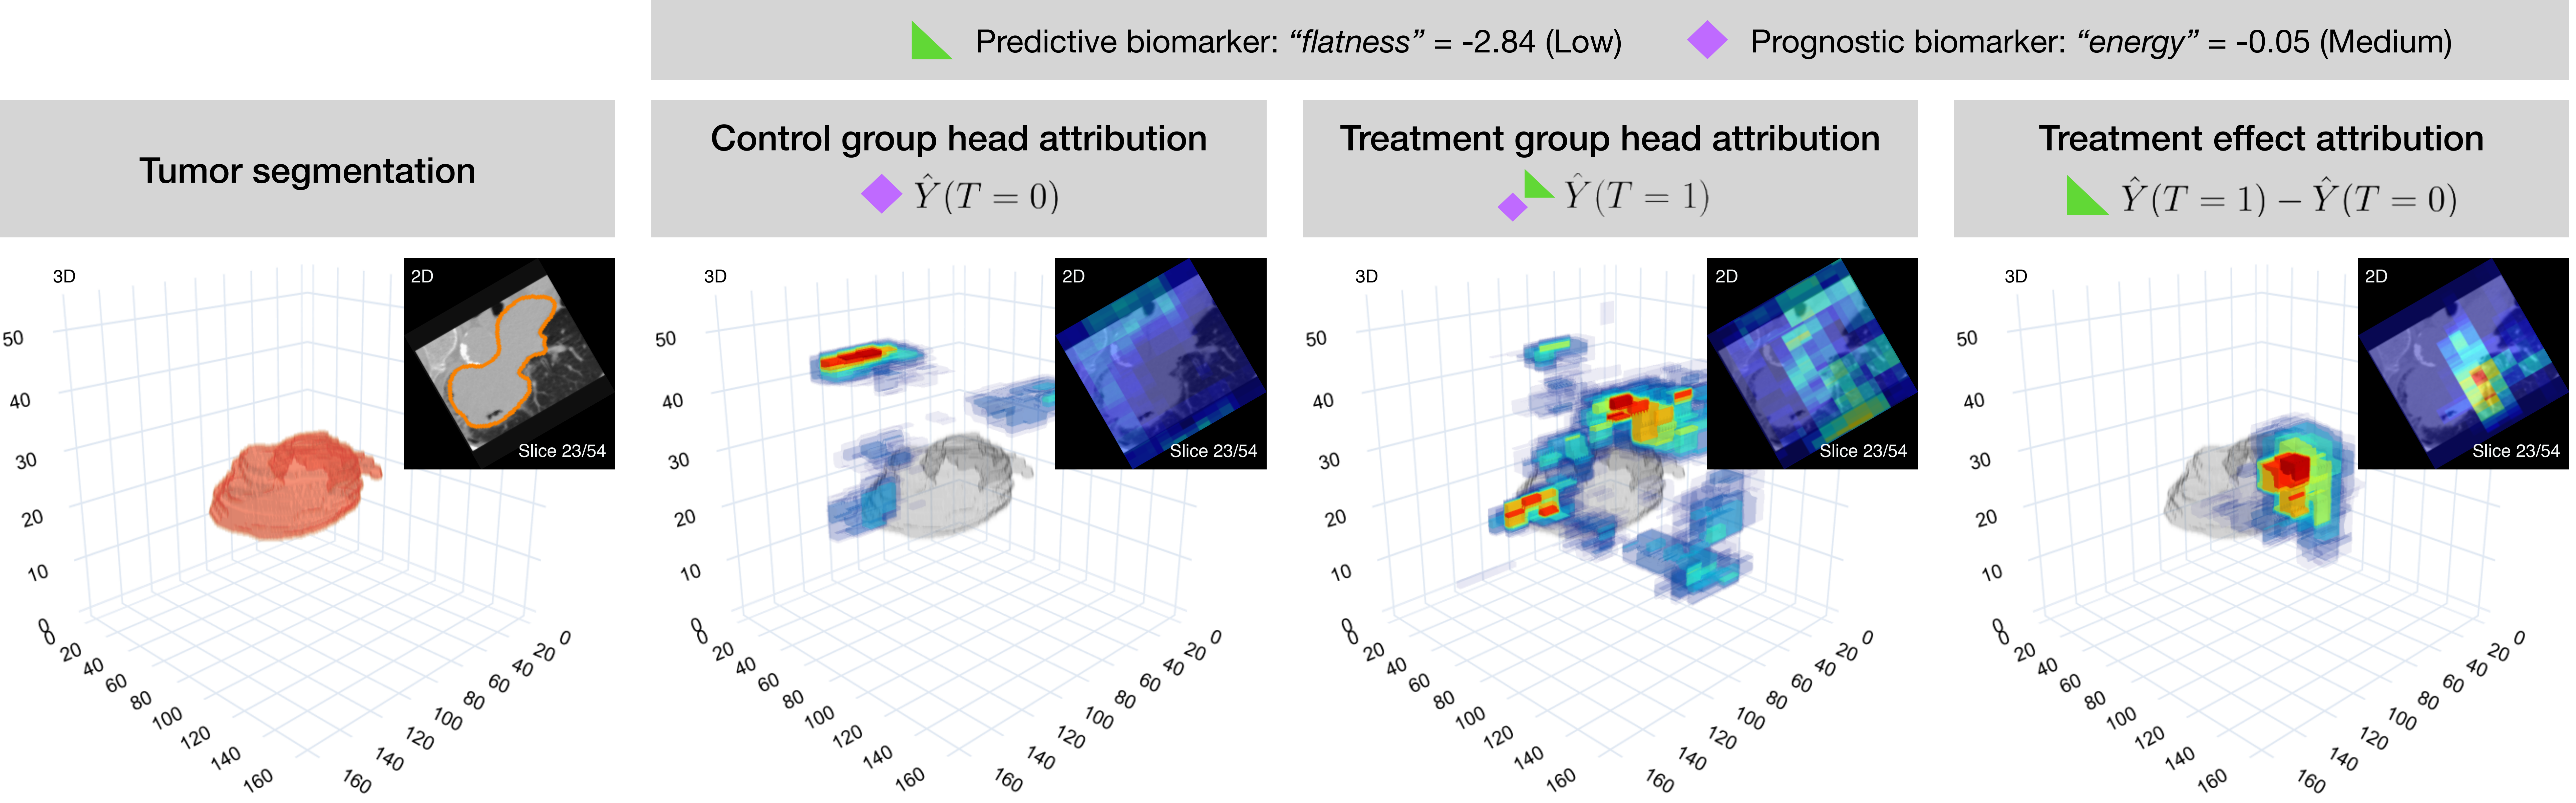
Predictive biomarker: "flatness" = -2.84 (Low)
Prognostic biomarker: "energy" = -0.05 (Medium)
Tumor segmentation
Control group head attribution
$\hat{Y}(T=0)$
Treatment group head attribution
$\hat{Y}(T=1)$
Treatment effect attribution
$\hat{Y}(T=1) - \hat{Y}(T=0)$
3D
2D
Slice 23/54

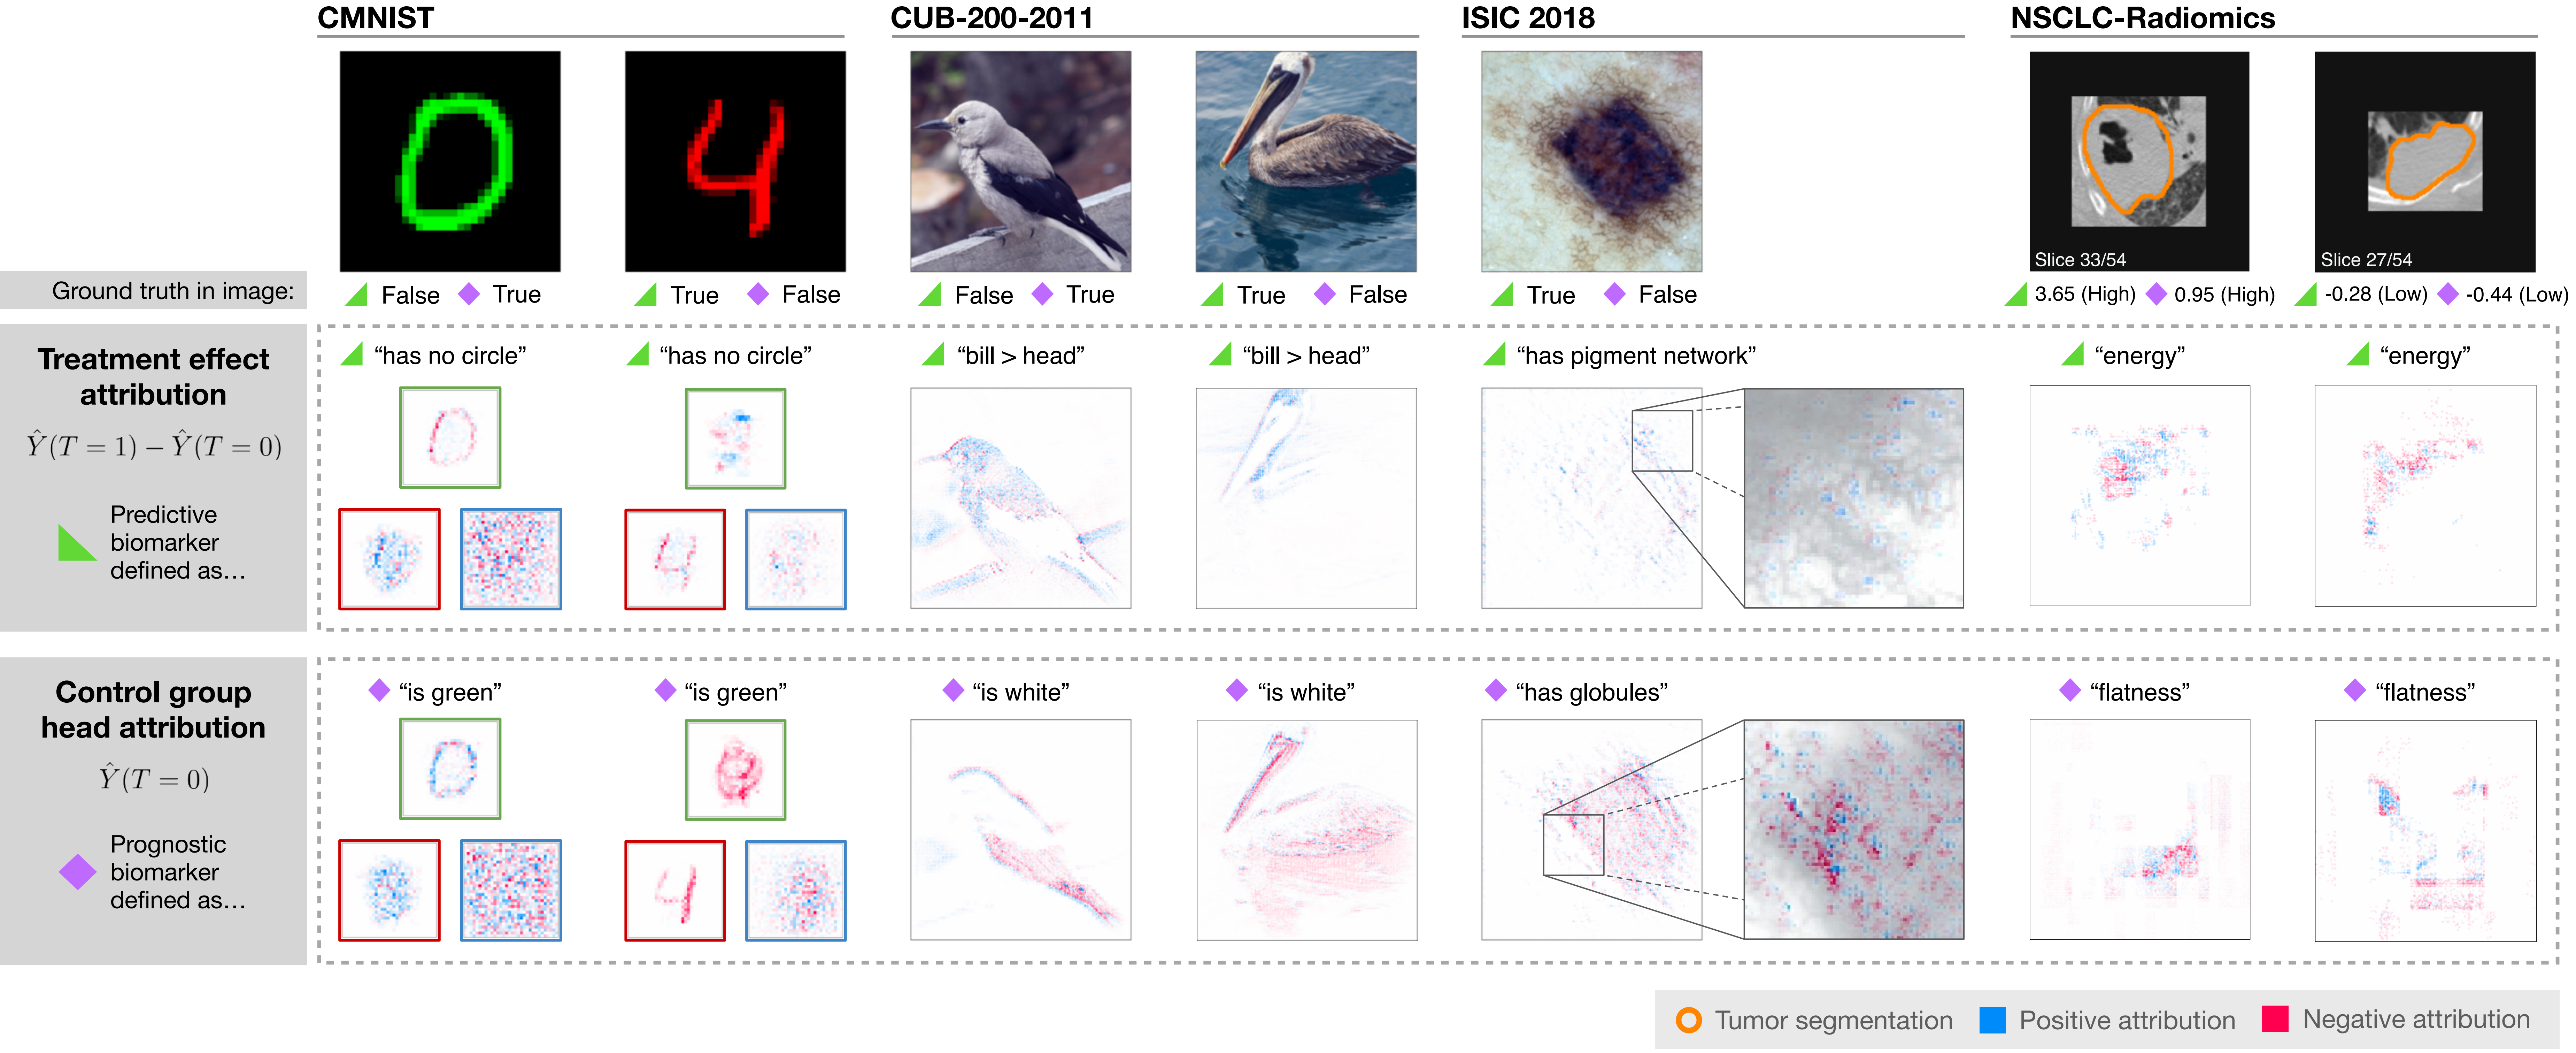

CMNIST
CUB-200-2011
ISIC 2018
NSCLC-Radiomics
Slice 33/54
Slice 27/54
Ground truth in image:
False True
True False
False True
True False
True False
3.65 (High) 0.95 (High)
-0.28 (Low) -0.44 (Low)
Treatment effect attribution
$\hat{Y}(T=1) - \hat{Y}(T=0)$
Predictive biomarker defined as…
"has no circle"
"has no circle"
"bill > head"
"bill > head"
"has pigment network"
"energy"
"energy"
Control group head attribution
$\hat{Y}(T=0)$
Prognostic biomarker defined as…
"is green"
"is green"
"is white"
"is white"
"has globules"
"flatness"
"flatness"
Tumor segmentation
Positive attribution
Negative attribution
